# Supplementary material for: AA-CLIP: Enhancing Zero-shot Anomaly Detection via Anomaly-Aware CLIP
Source: arXiv:2503.06661 source file (2025-03-09)
Supplement: Supplementary file 1 [file X_suppl.tex]

\clearpage
\clearpage
\setcounter{page}{1}
\maketitlesupplementary

This Supplementary Material contains the following three parts: 1) Additional Information about SOTA models, datasets and implementation details in \cref{sec:info}; 2) Additional experiments and further analysis about prompts, hyper-parameters, and data-efficient training in \cref{sec:add-exp}; 3) Pseudo-Code Implementation for \ourname in \cref{sec:pseudo}; 4) Additional visualization of image feature t-SNE and anomaly maps in \cref{sec:add-vis}.

\section{Additional Information}
\label{sec:info}
\subsection{SoTA Models}
To demonstrate the superiority of \ourname, we compare our methods with baseline CLIP~\cite{radford2021learning} and broad recent SoTA models. The introductions are given as follows:
\begin{itemize}
    \item{\textbf{CLIP}~\cite{radford2021learning}}, is a powerful multimodal model that learns to associate images and text through contrastive learning on large-scale datasets. By jointly training image and text encoders, CLIP can perform zero-shot classification, enabling it to understand and relate visual and textual information without task-specific fine-tuning.  We use the prompts in VAND~\cite{chen2023april} to generate predictions for anomaly detection tasks. 
    \item{\textbf{WinCLIP}~\cite{jeong2023winclip}}, published in CVPR 2023, enhances CLIP with a compositional ensemble of prompt templates and an efficient feature extraction method across image patches. It efficiently extracts and aggregates window/patch/image-level features to align with text, making progress in anomaly detection and segmentation tasks. The results of WinCLIP in our paper are copied from ~\cite{zhou2023anomalyclip,huang2024adapting}. 
    \item{\textbf{VAND}~\cite{chen2023april}} is a winning approach for the CVPR 2023 Zero/Few-shot Track of the Visual Anomaly and Novelty Detection (VAND) 2023 Challenge. It enhances CLIP with additional linear layers to map image features into a shared embedding space for anomaly map generation. The results of VAND in our paper is inferred from their official weights.
    \item{\textbf{MVFA-AD}~\cite{huang2024adapting}} is a work adapting CLIP to AD tasks, published in CVPR 2024. It proposes a multi-level adaptation framework to progressively refine image features. They mainly focus on medical domain in their original work. We re-train the model using the original code and original configuration to validate its generalization ability, except using VisA as training dataset. 
    \item{\textbf{AnomalyCLIP}~\cite{zhou2023anomalyclip}} is published in ICLR 2024, which is the first work targeting prompt-learning techniques to improve CLIP. It learns object-agnostic text prompts that capture general indicators of normality and abnormality, allowing the model to detect anomalies without being tied to specific object semantics. The results in our paper is inferred from the official weight.
    \item{\textbf{AdaCLIP}~\cite{cao2025adaclip}} published in ECCV 2024. It incorporates static and dynamic prompts allowing for shared and real-time adaptation, demonstrating strong zero-shot performance and generalization across diverse datasets. Their original implementation incorporates training in both industrial and medical datasets. We re-train the model with identical setting using VisA dataset.
\end{itemize}

\subsection{Datasets}
We conduct extensive experiments on ten public datasets from industrial and medical domains, covering five modalities. For each dataset, we use only the test set. Relevant details of the datasets are presented in \cref{tb:datasets}. 
\begin{table}[h]
	\centering
    \resizebox{\columnwidth}{!}{	
	\begin{tabular}{lccc|cc}
		\toprule
  \multirow{2}{*}{Dataset} & \multirow{2}{*}{Domain} & \multirow{2}{*}{Modalities} & \multirow{2}{*}{Classes} & \multicolumn{2}{c}{Number of Samples} \\
  \cline{5-6}
  &&&&Normal&Anomaly\\
  \midrule
  MVTec-AD & Industrial & Photography & 15 & 467 & 1258 \\
  MPDD & Industrial & Photography & 6 & 176 & 282 \\
  BTAD & Industrial & Photography & 3 & 451 & 290 \\
  \midrule
  Brain MRI & Medical & MRI & 1 & 640 & 1013 \\
  Liver CT & Medical & CT & 1 & 833 & 660 \\
  Retina OCT & Medical & OCT & 1 & 1041 & 764 \\
  ColonDB & Medical & Endoscopy & 1 & 0 & 380 \\
  ClinicDB & Medical & Endoscopy & 1 & 0 & 612 \\
  Kvasir & Medical & Endoscopy & 1 & 0 & 1000 \\
  CVC-300 & Medical & Endoscopy & 1 & 0 & 60 \\
	\bottomrule
	\end{tabular}
    }
    \vspace{-1.5mm}
	\caption{Key Information of The Datasets Used}
    \label{tb:datasets}
    \vspace{-1.5mm}
\end{table}

\subsection{Additional Implementation Details}
During training, all images are resized to $518 \times 518$ pixels. Data augmentation techniques—including color jitter, random rotation, random affine transformation, random horizontal flip, and random vertical flip—are applied with a probability of 0.5. Additionally, the default normalization of OpenCLIP is applied to all datasets during both training and inference. The hyper-parameters for Adam optimizer are set to $\beta_1=0.5,\ \beta_2=0.999$, following previous work~\cite{huang2024adapting}. For the first stage, the batch size is set to 16, while for the second stage, the batch size is 2. 

\subsection{Prompts}
\label{sec:prompts-details}
The prompt templates and descriptors we use are listed in \cref{tb:prompts-templates}. During both training and inference, ``[CLS]'' is replaced with the class description, and normal or anomaly descriptors are inserted into the templates. Normal and anomaly anchors are generated by averaging the embeddings of different prompts.
\begin{table}[h]
	\centering
    \resizebox{0.65\columnwidth}{!}{	
	\begin{tabular}{l|l}
		\toprule
  State & Prompt \\
  \midrule
  \multirow{2}{*}{Prompt Template} & \{\} \\
  & a photo of a \{\} \\
  \midrule
  \multirow{3}{*}{Normal Descriptors} & [CLS]\\
  & a [CLS]\\
  & the [CLS]\\
  \midrule
\multirow{5}{*}{Anomaly Descriptors} & damaged [CLS]\\
  & broken [CLS]\\
  & [CLS] with flaw \\
  & [CLS] with defect \\
  & [CLS] with damage\\
 	\bottomrule
	\end{tabular}
    }
    \vspace{-1.5mm}
	 \caption{Templates of Prompts Used}
 \label{tb:prompts-templates}
    \vspace{-1.5mm}
\end{table}

Considering the setting of AD aims to identify anomalies without prior knowledge of the specific anomaly types, we use only general adjectives to represent anomaly semantics, as shown in \label{tb:prompts}(Bottom). To describe a class, we utilize GPT-4 to automatically generate descriptions. Notably, only normal samples are input to GPT-4 to ensure proper generation, as shown in \cref{fig:gpt}.
{\small 
\begin{figure}[!t]
    \centering
    \includegraphics[width=0.9\linewidth]{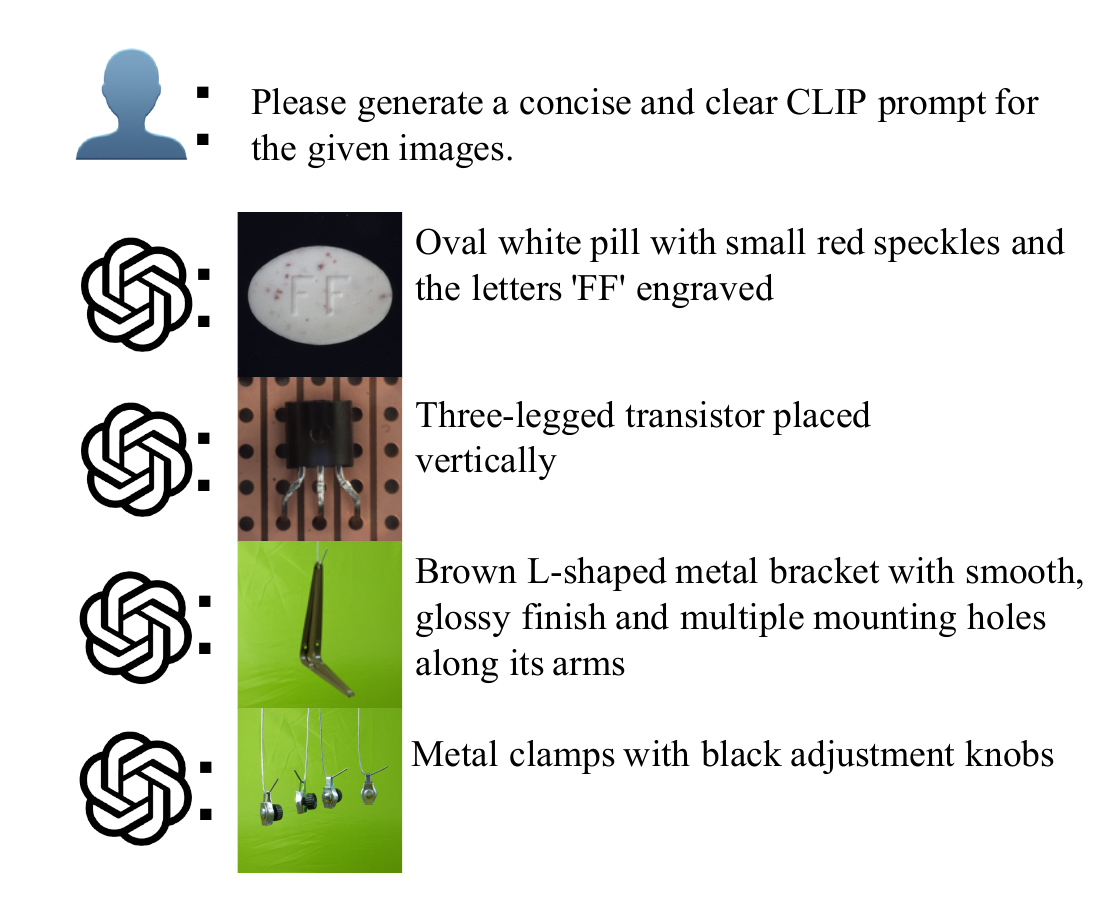}
    \vspace{-2.5mm}
    \caption{Examples of GPT-4 Generated Class Discription.}
    \label{fig:gpt}
\end{figure}
}

\section{Additional Experiments}
\label{sec:add-exp}
\begin{figure*}[t]
    \centering
    \includegraphics[width=\linewidth]{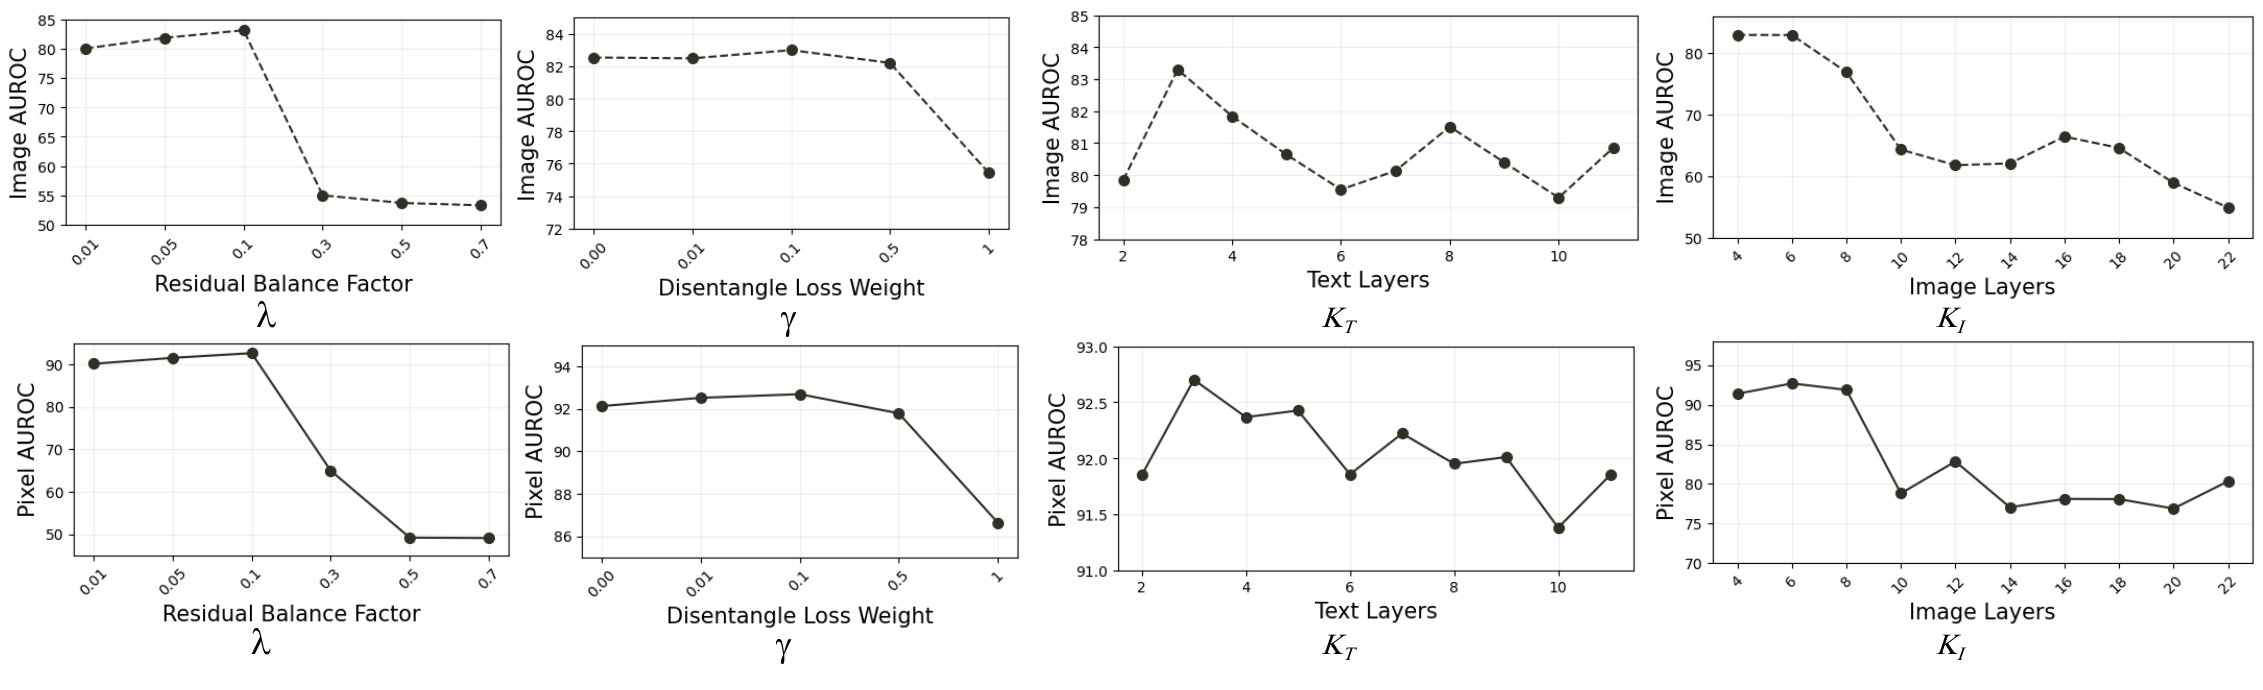}
    \caption{Ablation Study of Hyper-parameters}
    \label{fig:ablations}
\end{figure*}
\subsection{Prompts}
\label{sec:prompts}
\subsubsection{Templates}
To demonstrate the robustness of our model across various prompt templates, we present additional experimental results in \cref{tb:ab-templates}. We obtain inference results from the full-shot trained model using both seen and unseen prompt templates, testing on the BTAD and Retina OCT datasets. The results with novel prompt templates indicate that the effectiveness in differentiating anomalies is not dependent on the specific prompt templates used.
\begin{table}[h]
	\centering
    \resizebox{\columnwidth}{!}{	
	\begin{tabular}{ll|cc|cc}
		\toprule
  		\multicolumn{2}{c|}{\multirow{2}{*}{Prompt}} & \multicolumn{2}{c|}{BTAD} & \multicolumn{2}{c}{Retina OCT} \\
  		& & Pixel & Image & Pixel & Image \\
  		\midrule
        \multirow{2}{*}{Seen} & \{\}. & 97.0 & 94.7 & 95.5 & 82.7 \\
        & a photo of \{\}. & 97.4 & 94.8 & 95.6 & 82.7 \\
        \midrule
        \multirow{5}{*}{Unseen} & a picture of \{\}. & 97.3 & 94.6 & 95.4 & 82.3 \\
        & this is a photo of \{\}. & 97.3 & 94.6 & 95.7 & 82.4 \\
        & there is a \{\}. & 97.2 & 95.1 & 95.6 & 82.3 \\
        & a \{\} in the scene. & 96.7 & 95.4 & 95.6 & 82.1 \\
        & a close-up photo of \{\}. & 97.3 & 94.7 & 95.6 & 82.4 \\
 		\bottomrule
	\end{tabular}
    }
    \vspace{-1.5mm}
	\caption{AUROC Results of Different Prompt Templates Used}
    \vspace{-1.5mm}
	\label{tb:ab-templates}
\end{table}

\subsubsection{Anomaly Semantics}
To demonstrate that our model successfully learns generalizable anomalous semantics, we present additional experimental results using different anomaly descriptors in \cref{tb:ab-anomaly}, including seen and unseen ones. We obtain inference results from the full-shot trained model using both seen and unseen anomaly descriptors on the MPDD and Retina OCT datasets as examples. The results with novel anomaly descriptors indicate that the effectiveness in differentiating anomalies is not dependent on the specific adjectives used to describe anomaly in the prompts, further validating that our model successfully equips CLIP with anomaly-awareness.
\begin{table}[h]
	\centering
    \resizebox{\columnwidth}{!}{	
	\begin{tabular}{ll|cc|cc}
		\toprule
  		\multicolumn{2}{c|}{\multirow{2}{*}{Prompt}} & \multicolumn{2}{c|}{MPDD} & \multicolumn{2}{c}{Retina OCT} \\
  		& & Pixel & Image & Pixel & Image \\
  		\midrule
        \multirow{5}{*}{Seen} & damaged [CLS] & 96.6 & 75.0 & 95.4 & 81.8 \\
        & broken [CLS] & 96.8 & 75.1 & 95.4 & 82.6 \\
        & [CLS] with flaw & 96.7 & 75.6 & 94.6 & 82.8 \\
        & [CLS] with defect & 96.6 & 75.3 & 95.6 & 82.6 \\
        & [CLS] with damage & 96.5 & 75.4 & 95.4 & 82.6 \\
        \midrule
        \multirow{6}{*}{Unseen} & corrupted [CLS] & 94.3 & 72.9 & 93.3 & 82.5 \\
        & defective [CLS] & 96.4 & 75.1 & 95.5 & 82.9 \\
        & flawed [CLS] & 96.6 & 74.4 & 95.5 & 82.6 \\
        & impaired [CLS] & 96.7 & 75.5 & 94.9 & 80.9 \\
        & [CLS] with defective parts & 96.1 & 73.0 & 95.2 & 81.7 \\
        & [CLS] with damaged parts & 97.1 & 73.0 & 95.4 & 81.5 \\
 		\bottomrule
	\end{tabular}
    }
    \vspace{-1.5mm}
	\caption{AUROC Results of Different Anomaly Descriptors Used}
    \vspace{-1.5mm}
	\label{tb:ab-anomaly}
\end{table}

\subsection{Additional Ablations for Hyper-parameters}

We provide additional results of different hyper-parameter settings in this section, as shown in \cref{fig:ablations}. The hyper-parameters include:
\begin{itemize}
    \item $\lambda$ controls the residual fusing ratio,
    \item $\gamma$ controls the weight of Disentangle Loss $L_{dis}$,
    \item $K_T/K_I$ controls layers of inserted adapters in text/visual encoder.
\end{itemize}

A large residual ratio $\lambda$ means that the output contains less information from CLIP and more information from linear adapter, allowing more flexible adaptation and leading to improvement when $\lambda\leq0.1$. However, due to the modeling limitation and catastrophic forgetting, zero-shot performance drops dramatically after $\lambda\geq 0.3$.

Since $L_{dis}$ is a normalization loss without information flowing from training data, a large $\gamma$ can be detrimental to the learning process because of semantic disturbance to CLIP's feature space, leading to performance drop.

For $K_T/K_I$, inserting adapters in shallow layers prevents drastic semantic changes caused by inserting adapters in deep layers and maintains training stability. Large $K_T/K_I$ damages overall performance significantly because of higher possibility of catastrophic forgetting with more trainable parameters.
Since it contains more semantically meaningful information in text space, the performance fluctuation for text encoder is more obvious compared to image encoder.

\subsection{Comparison under Various Data Levels}
We re-implement SOTA methods for comparison under different settings: 2-shot per class, 16-shot per class, 64-shot per class, and full-shot, presented in line-figure format. In addition to the BTAD results shown in our main paper, additional figures are displayed in  \cref{fig:plots}. Our method demonstrates relatively stable superiority across all methods, maintaining a leading position in most scenarios. These results prove that our training strategy has high fitting efficiency.
{\small 
\begin{figure}[!t]
    \centering
    \includegraphics[width=0.9\linewidth]{img/visualization/plot.pdf}
    \vspace{-2.5mm}
    \caption{Additional Results under Different Data Levels}
    \label{fig:plots}
\end{figure}
}

Despite notable domain gaps among test datasets, which can cause some variability in results, our model’s performance generally improves as training data increases, with minor fluctuations. We provide an explanation as follows: with limited data, the adapted image encoder initially leverages textual cues, effectively identifying anomalies while occasionally leading to false positives. As more data becomes available, the model captures richer and more balanced features, further enhancing accuracy. However, with excessive data, the model may start to capture domain-specific details over broader abnormality semantics, reducing generalization to unseen anomalies. This trend aligns with our visualizations and is consistent across our implementations of other methods, leaving space for further investigation on stable adaptation.

\section{Pseudocode Implementation for \ourname}
\label{sec:pseudo}
To clearly demonstrate AA-CLIP model, we present our model definition using PyTorch-style pseudocode, as shown ~\cref{fig:pseudocode}. 
{\small 
\begin{figure}[h]
    \centering
    \includegraphics[width=0.9\linewidth]{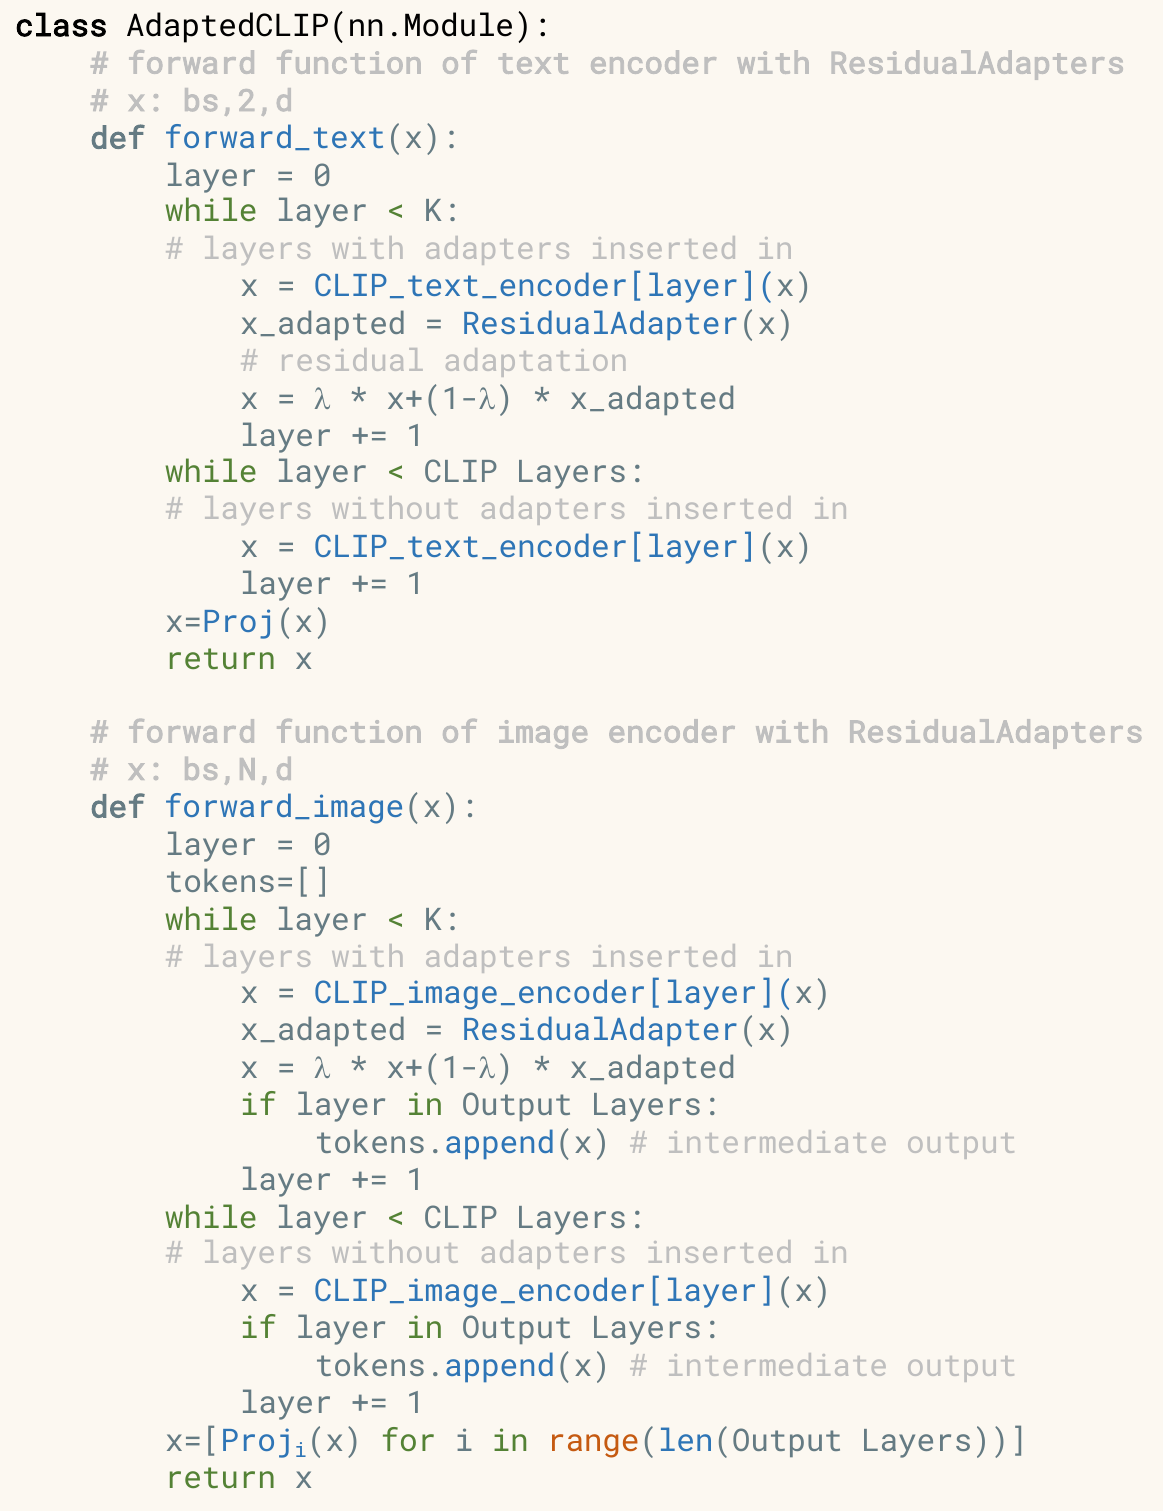}
    \vspace{-2.5mm}
    \caption{Pseudocode Implementation of AA-CLIP}
    \label{fig:pseudocode}
\end{figure}
}

\section{Additional Visualization}
\label{sec:add-vis}
\subsection{Image t-SNE Visualization}
In our main paper, we present t-SNE visualizations for text embeddings of both seen and unseen classes. Additionally, we include further visualizations of image features for seen classes in \cref{fig:ab-tsne-seen} and for unseen classes in \cref{fig:ab-tsne-unseen}. The results for original CLIP and AA-CLIP are from same t-SNE optimization iterations. We keep the number of normal and anomaly patches the same for clear visualization. The results prove that our model succeed in equipping CLIP with generalizable anomaly discrimination ability.

\subsection{Anomaly Maps Visualization}
{\small 
\begin{figure}[h]
    \centering
    \includegraphics[width=\linewidth]{img/visualization/MVTec.pdf}
    \vspace{-2.5mm}
    \caption{Additional Visualization Examples of AnomalyCLIP and AA-CLIP.}
    \label{fig:MVTec}
\end{figure}
}
{\small 
\begin{figure}[h]
    \centering
    \includegraphics[width=\linewidth]{img/visualization/BTAD.pdf}
    \vspace{-2.5mm}
    \caption{Additional Visualization Examples of AnomalyCLIP and AA-CLIP.}
    \label{fig:BTAD}
\end{figure}
}
{\small 
\begin{figure*}[t]
    \centering
    \includegraphics[width=\linewidth]{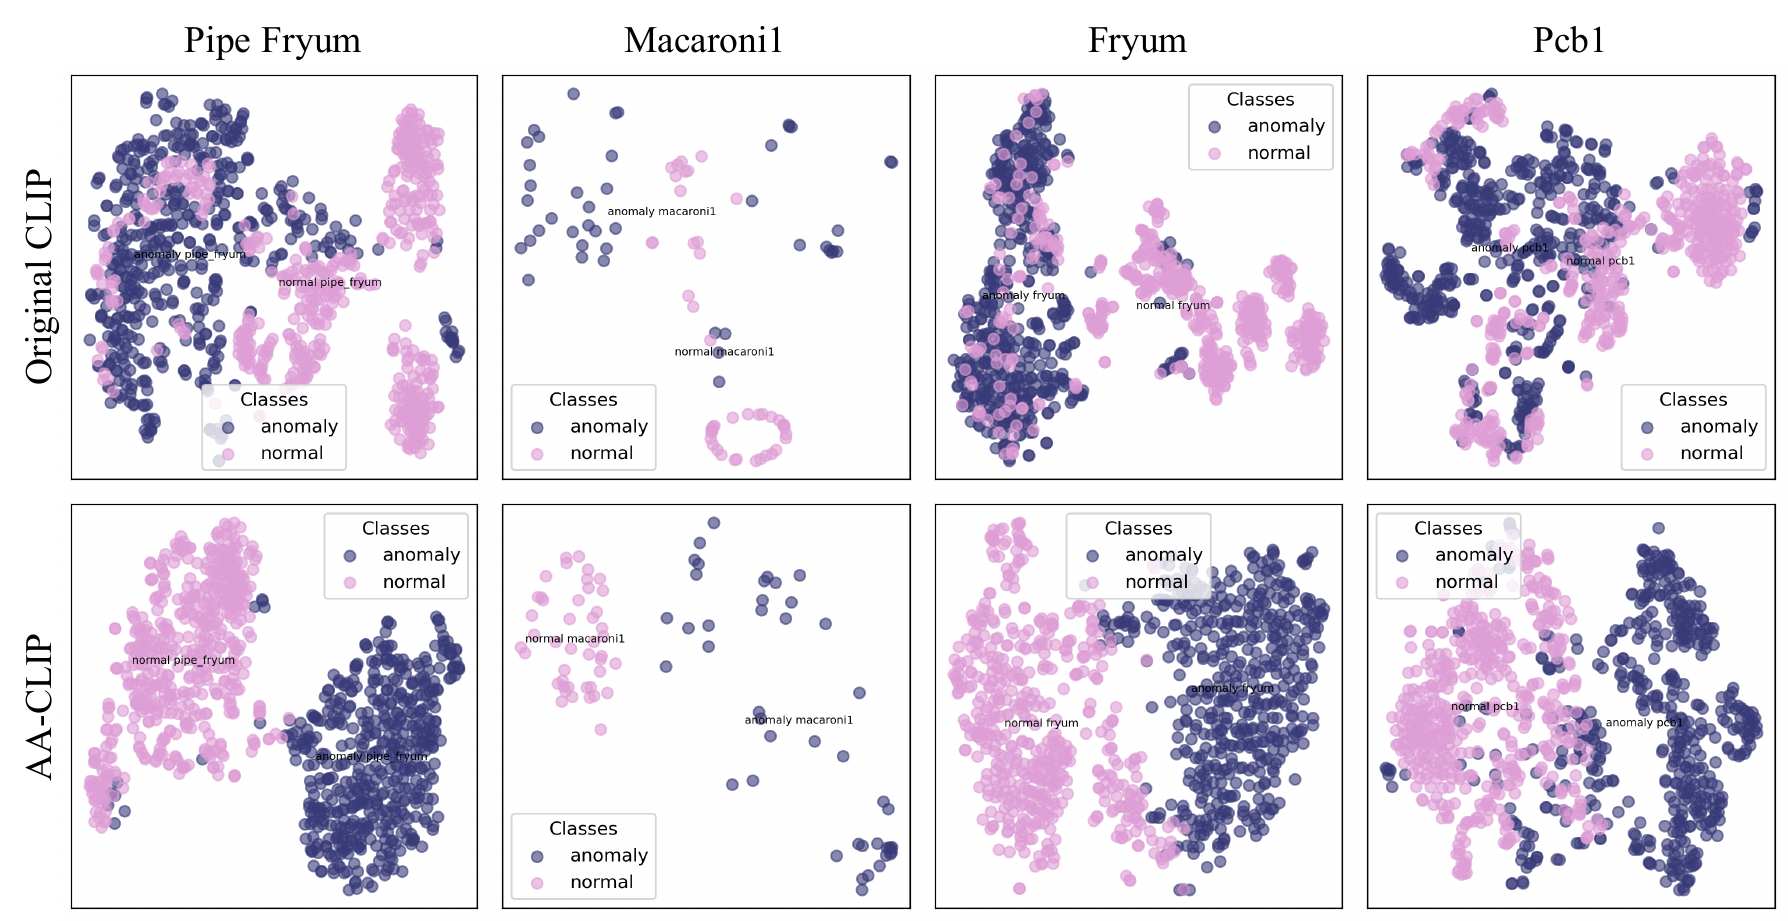}
    \vspace{-2.5mm}
    \caption{Additional t-SNE Visualization of Visual Features of Seen Classes}
    \label{fig:ab-tsne-seen}
\end{figure*}
}
{\small 
\begin{figure*}[t]
    \centering
    \includegraphics[width=\linewidth]{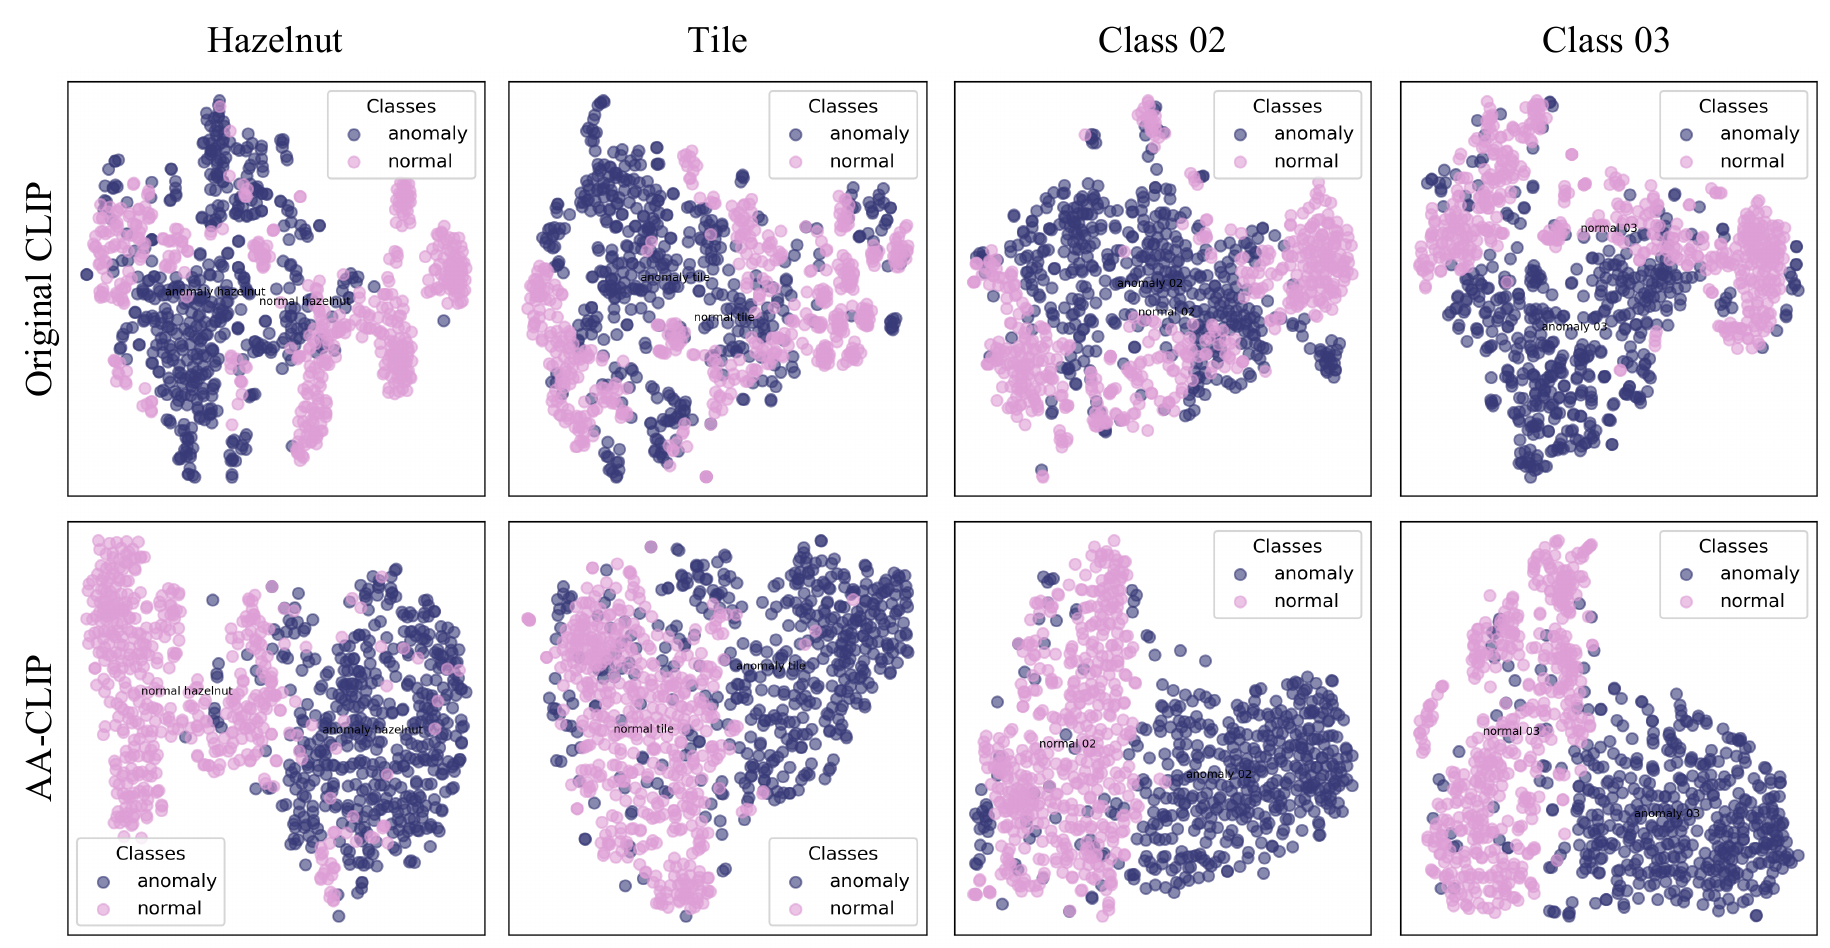}
    \vspace{-2.5mm}
    \caption{Additional t-SNE Visualization of Visual Features of Unseen Classes}
    \label{fig:ab-tsne-unseen}
\end{figure*}
}
We provide additional visualization examples of \ourname to illustrate the effectiveness of our method. We show more comparative results of recent SOTA AnomalyCLIP and our methods in \cref{fig:MVTec,fig:BTAD}. Despite AnomalyCLIP can identify anomalous regions, our model's predictions have less false-positive predictions and localizes anomalous regions more precisely.

We provide more examples of our AA-CLIP's prediction, as shown in \cref{fig:bottle,fig:capsule,fig:grid,fig:carpet,fig:hazelnut,fig:zipper,fig:toothbrush,fig:tubes,fig:brain,fig:retina,fig:colon,fig:cvc300}. For each figure, the first row shows the input, with anomaly regions highlighted in red in the second row. The final row displays the segmentation results generated by \ourname. Our model shows precise localization results in general.
{\small 
\begin{figure*}[!t]
    \centering
    \includegraphics[width=\linewidth]{img/visualization/bottle.pdf}
    \vspace{-2.5mm}
    \caption{Visualization Examples of Class Bottle in MVTec-AD dataset.}
    \label{fig:bottle}
\end{figure*}
}
{\small 
\begin{figure*}[!t]
    \centering
    \includegraphics[width=\linewidth]{img/visualization/capsule.pdf}
    \vspace{-2.5mm}
    \caption{Visualization Examples of Class Capsule in MVTec-AD dataset.}
    \label{fig:capsule}
\end{figure*}
}
{\small 
\begin{figure*}[!t]
    \centering
    \includegraphics[width=\linewidth]{img/visualization/grid.pdf}
    \vspace{-2.5mm}
    \caption{Visualization Examples of Class Grid in MVTec-AD dataset.}
    \label{fig:grid}
\end{figure*}
}
{\small 
\begin{figure*}[!t]
    \centering
    \includegraphics[width=\linewidth]{img/visualization/carpet.pdf}
    \vspace{-2.5mm}
    \caption{Visualization Examples of Class Carpet in MVTec-AD dataset.}
    \label{fig:carpet}
\end{figure*}
}
{\small 
\begin{figure*}[!t]
    \centering
    \includegraphics[width=\linewidth]{img/visualization/hazelnut.pdf}
    \vspace{-2.5mm}
    \caption{Visualization Examples of Class Hazelnut in MVTec-AD dataset.}
    \label{fig:hazelnut}
\end{figure*}
}
{\small 
\begin{figure*}[!t]
    \centering
    \includegraphics[width=\linewidth]{img/visualization/zipper.pdf}
    \vspace{-2.5mm}
    \caption{Visualization Examples of Class Zipper in MVTec-AD dataset.}
    \label{fig:zipper}
\end{figure*}
}
{\small 
\begin{figure*}[!t]
    \centering
    \includegraphics[width=\linewidth]{img/visualization/toothbrush.pdf}
    \vspace{-2.5mm}
    \caption{Visualization Examples of Class Toothbrush in MVTec-AD dataset.}
    \label{fig:toothbrush}
\end{figure*}
}
{\small 
\begin{figure*}[!t]
    \centering
    \includegraphics[width=\linewidth]{img/visualization/tubes.pdf}
    \vspace{-2.5mm}
    \caption{Visualization Examples of Class Tubes in MPDD dataset.}
    \label{fig:tubes}
\end{figure*}
}
{\small 
\begin{figure*}[!t]
    \centering
    \includegraphics[width=\linewidth]{img/visualization/brain.pdf}
    \vspace{-2.5mm}
    \caption{Visualization Examples of Brain MRI dataset.}
    \label{fig:brain}
\end{figure*}
}
{\small 
\begin{figure*}[!t]
    \centering
    \includegraphics[width=\linewidth]{img/visualization/retina.pdf}
    \vspace{-2.5mm}
    \caption{Visualization Examples of Retina OCT dataset.}
    \label{fig:retina}
\end{figure*}
}
{\small 
\begin{figure*}[!t]
    \centering
    \includegraphics[width=\linewidth]{img/visualization/clinicDB.pdf}
    \vspace{-2.5mm}
    \caption{Visualization Examples of endoscopic photos in ClinicDB dataset.}
    \label{fig:colon}
\end{figure*}
}
{\small 
\begin{figure*}[!t]
    \centering
    \includegraphics[width=\linewidth]{img/visualization/cvc300.pdf}
    \vspace{-2.5mm}
    \caption{Visualization Examples of endoscopic photos in CVC-300 dataset.}
    \label{fig:cvc300}
\end{figure*}
}
